# Supplementary material for: Cross-phase modulation in the two dimensional spectroscopy
Source: arXiv:2308.01396 source file (2023-08-02)
Supplement: Supplementary file 1 [file Supp_TwoDES_XPM_04.pdf]

# Supplementary

Mao-Rui Cai,[1] Xue Zhang,[1] Zi-Qian Cheng,[1] Teng-Fei Yan,[2,*] and Hui Dong[1,†]

[1] *Graduate School of China Academy of Engineering Physics, No. 10 Xibeiwang East Road, Haidian District, Beijing 100193, China*

[2] *School of Microelectronics, shanghai university, Shanghai 200444, China*

Due to the possible non-uniform distribution of the frequency components in the transverse plane (i.e., the spatial chirp), the spectrum of the pump pulse detected by the spectrometer may not represent the actual spectrum evolved in the XPM process. Hence, instead of directly detecting the spectrum of the pump pulse with a spectrometer, we determine the parameters of the pump pulse by simulating the 2DCS-XPM and Gaussian fittings its projection trace on the axis of $\omega_\tau$.

Our procedure starts by projecting all the measured 2DCS-XPMs (with $T$ scanned from -100 fs to 30 fs) onto the axis of $\omega_\tau$. These projections are then averaged and fitted with a Gaussian function of the form $f(\omega_\tau) = C_0 \exp\left\{-0.5\left(\omega_\tau - \omega_{\text{prjct}}\right)^2/\sigma_{\text{prjct}}^2\right\} + C_1$. The results of the experiments conducted without and with ASW are depicted in Fig.1(a) and (b), respectively. The fitting outcomes are $\omega_{\text{prjct}}^{e1}/2\pi = 449.59$ THz, $\sigma_{\text{prjct}}^{e1}/2\pi = 6.00$ THz for the experiment without the additional SW, and $\omega_{\text{prjct}}^{e2}/2\pi = 449.19$ THz, $\sigma_{\text{prjct}}^{e2}/2\pi = 5.96$ THz for the experiment with the additional SW on the probe arm.

According to Eq. (21) in the main text, the XPM is centered at $\omega_\tau = \Omega_1$, which corresponds to the central frequency of the pump pulse. Therefore, the central frequency of the pump pulse $\Omega_1$ is directly determined by $\omega_{\text{prjct}}$. Specially, in this case, $\Omega_1^{e1}/2\pi = \omega_{\text{prjct}}^{e1}/2\pi = 449.59$ THz and $\Omega_1^{e2}/2\pi = \omega_{\text{prjct}}^{e2}/2\pi = 449.19$ THz. However, it is not apparent (from these projections) what the duration of the pump pulse $\tau_1$ is, as the bandwidth of the projection $\sigma_{\text{prjct}}$ differs from the bandwidth of the pump pulse $\sigma_1 = 1/\tau_1$.

To determine the duration of the pump pulses, we perform numerical simulations of the 2DCS-XPM with $T$ scanned from -100 fs to 30 fs. In our simulations, we specifically scan $\tau_1$ from 25 fs to 75 fs, while keeping other pulse parameters based on the experimental results. For instance, we adopt values $\Omega_3/2\pi = 438.09$ THz, $\tau_{3,0} = 13.56$ fs, $\beta_{gdd}^{e1} = 613.76\,\text{fs}^2$

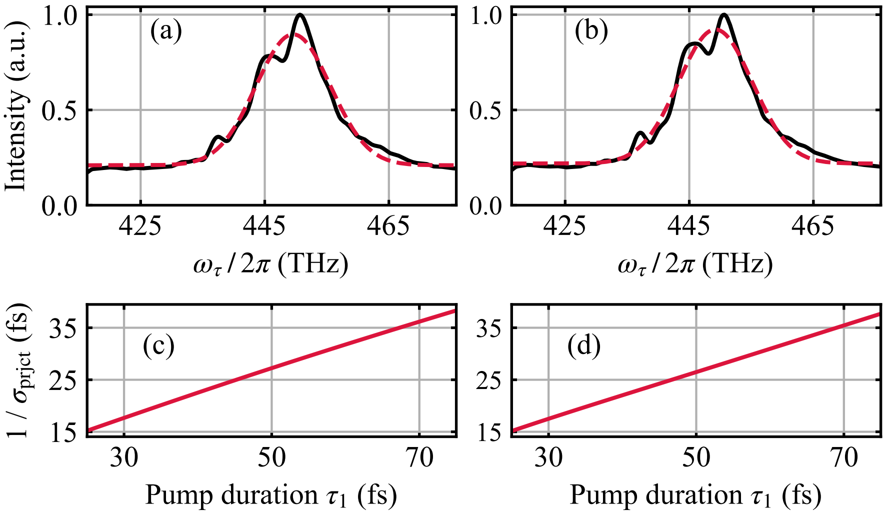


Figure 1. (a, b) Projections of experimental 2DCS-XPMs onto the axis of $\omega_\tau$, and (c, d) bandwidths of the projections as functions of $\tau_1$. In (a) and (b), the black solid lines represent the averaged projections obtained from the experimental measurements of 2DCS-XPMs, with T scanned from -100 fs to 30 fs. The red dash lines represent the corresponding Gaussian fittings, with central frequencies $\omega_{\text{prjct}}^{e1}/2\pi = 449.59$ THz, $\omega_{\text{prjct}}^{e2}/2\pi = 449.19$ THz and bandwidths $\sigma_{\text{prjct}}^{e1}/2\pi = 6.00$ THz, $\sigma_{\text{prjct}}^{e2}/2\pi = 5.96$ THz, respectively. In (c) and (d), the reciprocal of the bandwidths of the projections is approximately linear with pump duration $\tau_1$.

* yantf@shu.edu.cn

† hdong@gscaep.ac.cn

and $\Omega_1^{e_1}/2\pi = 449.59$ THz for simulating the results without SW. For simulating the results with SW, we use values $\Omega_3/2\pi = 438.09$ THz, $\tau_{3,0} = 13.56$ fs, $\Omega_1^{e_2}/2\pi = 449.19$ THz and $\beta_{gdd}^{e_2} = 882.79$ fs$^2$. Subsequently, similar with the procedure we conducted in Fig.1(a) and (b), the simulated 2DCS-XPMs are projected onto the axis of $\omega_\tau$, and the projections are averaged with respect to $T$ and Gaussian fitted to yield a corresponding bandwidth $\sigma_{\mathrm{prjct}}$.

Through these simulations, we discover the reciprocal relation between the bandwidth of the projection and the duration of the pump pulse. This relation is illustrated in Fig.1(c) and (d), where we plot $1/\sigma_{\mathrm{prjct}}$ as a function of $\tau_1$. By performing linear fitting on Fig.1(c) and (d) and with the experimental bandwidth of the projection, $\sigma_{\mathrm{prjct}}^{e_1}/2\pi = 6.00$ THz and $\sigma_{\mathrm{prjct}}^{e_2}/2\pi = 5.96$ THz, we obtain the optimal pump duration $\tau_1^{e_1} = 48.85$ fs for the experiment without SW and $\tau_1^{e_2} = 50.48$ fs for the experiment with SW.
